# Supplementary material for: Adaptive Density Estimation for Generative Models
Source: arXiv:1901.01091 source file (2020-01-03)
Supplement: Supplementary file 2 [file latex_tile.tex]

\setlength{\tabcolsep}{0pt}
\begin{tabular}{cccc} 
\includegraphics{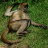} &
\includegraphics{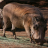} &
\includegraphics{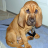} &
\includegraphics{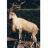}\\[-0.85ex]
\includegraphics{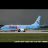} &
\includegraphics{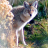} &
\includegraphics{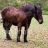} &
\includegraphics{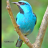}\\[-0.85ex]
\includegraphics{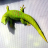} &
\includegraphics{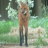} &
\includegraphics{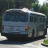} &
\includegraphics{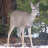}\\[-0.85ex]
\includegraphics{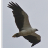} &
\includegraphics{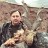} &
\includegraphics{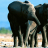} &
\includegraphics{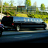}\\[-0.85ex]
\includegraphics{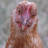} &
\includegraphics{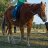} &
\includegraphics{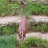} &
\includegraphics{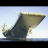}\\[-0.85ex]
\includegraphics{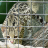} &
\includegraphics{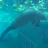} &
\includegraphics{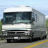} &
\includegraphics{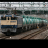}\\[-0.85ex]
\includegraphics{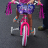} &
\includegraphics{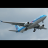} &
\includegraphics{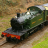} &
\includegraphics{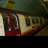}\\[-0.85ex]
\includegraphics{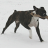} &
\includegraphics{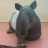} &
\includegraphics{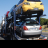} &
\includegraphics{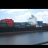}\\[-0.85ex]
\includegraphics{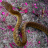} &
\includegraphics{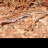} &
\includegraphics{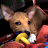} &
\includegraphics{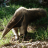}\\
\end{tabular}
